# Supplementary material for: Integrative Modeling and Analysis of the Interplay Between Epidemic and News Propagation Processes
Source: arXiv:2303.04441 source file (2023-03-08)
Supplement: Supplementary file 1 [file Appendix_SA.tex]

\newpage
\onecolumn 
\section*{Appendix A}

{\bf Theorem 1:} %We will apply 
%\cite[Theorem9]{[Applications of Mathematics 22] Albert Benveniste, Michel MÃ©tivier, Pierre Priouret (auth.) - Adaptive Algorithms and Stochastic Approximations (1990, Springer-Verlag Berlin Heidelberg) - libgen.lc.pdf} to prove this.
Towards this we need to prove the   properties listed below:

%{\it Assumptions of Benevenste.et.al}

We state the assumptions  in our notations:
\begin{enumerate}[{\bf B}.1]
    \item 
 There exists a family ${P_\phi}$ of transition probabilities ${P_\phi (\xi, A)}$ such that, for any Borel subset A we have
\begin{eqnarray}
P[\xi_
{n+1} \in A \mid \mathcal{F}_n] = P_{\phi_n}(\xi_n, A)
\end{eqnarray}

where $\mathcal{F}_n = \sigma(\phi_0, \xi_0, \xi_1, · · · , \xi_k)$ is a sigma algebra . This in turn implies that
the tuple $(\xi_k, \phi_k)$ forms a Markov chain.\newline

\item  For any compact subset Q of D, there exist constants $C_1, q_1$ such that for all $\phi \in D$  we have
\begin{eqnarray}
\|H_1 (\xi, \phi)\| \le C_1 (1+ | \xi|^{q_1}).
\end{eqnarray}

\item  There exists a function $h_1$ on D, and for each $\phi \in D$ a function $\nu_\phi (.)$ such that
\begin{enumerate}
    \item $h_1$  is locally Lipschitz on D.
    \item $(I - P_{\phi}) \nu_{\phi} (\xi) = H_1 (\xi, \phi) - h_1 (\phi)$, where $I$ is Identity matrix of same order as of $P_{\phi}$.
    \item For all compact set Q of D, there exist constants $C_3, C_4, q_3, q_4$ and $\lambda \in [0.5,1]$, such that for all $\phi , \phi' \in Q$
\end{enumerate}
 
\begin{eqnarray}
i. \| \nu_\phi (\xi)\| \le C_3 (1+ | \xi |^{q_3}),
\end{eqnarray}\\.
 \begin{eqnarray}
ii. \| P_\phi \nu_\phi (\xi) - P_\phi' \nu_\phi' (\xi)\| \le C_4 (1+ | \xi |^{q_4}) \| \phi - \phi'\|^\lambda.
\end{eqnarray}\\.

\item  For any compact set Q in D and for any $q>0$ ,there exists a $\mu_q(Q)<\infty$ ,such that
for all n, $\xi, A = \phi \in R^d$
\begin{eqnarray}
E_{\xi, \phi} {I(\phi_k , \xi_k \in Q, k \le n) (1 + \|\xi_{n+1}\|^q)} \le \mu_q (Q) (1 + \|\xi_{n}\|^q),
\end{eqnarray},
where $E_{\xi, \phi}$ represents the expectation taken with initial conditions $(\xi_0 ,\phi_0) = (\xi , \phi)$.
\end{enumerate}

{\bf Proof of theorem:} We begin with assumption 
\begin{enumerate}[{\bf B}.1]
\item From equation %$\eqref{conditional_expectation}$,
clearly assumption is satisfied with
$$
P_{\phi_n} (\xi_n, A) = Q_{\theta_n} (A) \mbox{ where }  Q_{\theta_n} (A) := P ( \xi_{n+1} \in A | \theta_n )
$$
\item First observe that $H_1 (\xi, \phi)$  can be expressed as a vector as follows:
$$
H_1 (\xi, \phi) = \begin{bmatrix}
(\mathcal{J}_{\phi} (E[\xi / \theta] - \theta) + (1 - \mathcal{J}_{\phi})(-C\theta))\\
(\mathcal{J}_{\phi} (E[\xi / \theta] - \psi - 1) + (1 - \mathcal{J}_{\phi})(-\psi))\\

\end{bmatrix}
$$

which gives  \begin{eqnarray}
\|H_1 (\xi, \phi)\| \le \sup_{\phi \in D} \| \phi \| (1+ |\xi|)
\end{eqnarray}
and so q = 1.

     \item If we consider $\nu_\phi (\xi) = H_1 (\xi, \phi) \ and \ h_1 (\phi) = (P_{\phi})\nu_{\phi}  (\xi)$ to be defined as \\
\begin{eqnarray}
(P_{\phi})\nu_{\phi}  (\xi) =  \int H_1 (y, \phi)(Q_{\phi})dy
\end{eqnarray}, then
\begin{enumerate} [{\bf a.}]
    \item  As $| h_1 (\phi) - h_1(\phi')| \le (C + 1) |\theta - \theta'| + (\psi - \psi') + (E[\xi / \theta] - E[\xi / \theta'])$

 We can therefore conclude that $h_1$ is lipschiz based on assumption A.2.\\
    \item  The definitions of $h_1 (\phi)$ and $H_1(\xi, \phi)$ make this obvious.
    \item 
    \begin{enumerate}[i.)]
        \item As $\nu_\phi(\xi) = H_1 (\xi, \phi)  $ and also  
     \begin{eqnarray}
\|H_1 (\xi, \phi)\| \le \sup_{\phi \in D} \| \phi \| (1+ |\xi|)
\end{eqnarray}
  So, like component B.2, we can say that this is also bounded by $C_3 (1+ | \xi|^{q_3})$, \\
  where $C_3 = \sup_{\phi \in D}\| \phi \| \ \text{and} \ q = 1.$\\
   \item
  \begin{eqnarray}
 \| P_\phi \nu_\phi (\xi) - P_\phi' \nu_\phi' (\xi)\| = \|h_1(\phi) - h_1(\phi')\| \le (C + 1) |\theta - \theta'| + (\psi - \psi') + (E[\xi / \theta] - E[\xi / \theta']) =  C_4 (1+ | \xi |^{q_4}) .
\end{eqnarray}\\.
  \end{enumerate}
\end{enumerate}

Now for assumption ${\bf B}.4$
\begin{align*}
 E_{\xi, \phi} {I(\phi_k , \xi_k \in Q, k \le n) (1 + \|\xi_{n+1}\|^q)} &\le E_{\xi, \phi} {I(\phi_n , \xi_n \in Q) (1 + \|\xi_{n+1}\|^q)}\\
 &\le \sup_{\phi \in Q}  \int (1 + y^q) Q(\phi,dy)\\ 
 &= \sup_{\phi \in Q} E[1+\xi_{n+1}^q | \theta_n = \theta]\\ 
&= \mu_q (Q)\\
&= 1 + B^q.   
\end{align*}
\end{enumerate}
 \eop
 
 \ignore{
 \begin{eqnarray}
    \label{Eqn_beta_i1}
\beta(t) =  \beta (i(t) )&=&
\beta + \sum_{k:\eta_k = \ueta } w_k  \frac{ \ueta   (p i + q) }{ a \ueta (pi+q) + 1 }\\
&=&   
\beta + {\bar w}  \frac{ \ueta   (p i + q) }{ a \ueta (pi+q) + 1 }, \nonumber
\end{eqnarray}

 \begin{eqnarray}
\frac{di}{dt} &=& \beta (i) i (1-i) - \alpha i = i h(i). 
\end{eqnarray}

Thus
\begin{eqnarray*}
h(i) &=& \beta  (1-i) + {\bar w}  \frac{ \ueta   (p i + q) }{ a \ueta (pi+q) + 1 } (1-i) - \alpha  
\ = \  \beta -\alpha   -\beta i + {\bar w}  \frac{ \ueta   (p i + q) }{ a \ueta (pi+q) + 1 } (1-i)  
\\
&=& \frac{1}{a \ueta (pi+q) + 1} \Bigg (- i^2 (\beta a \ueta p + {\bar w} \ueta p ) + i \left (
  (\beta-\alpha) a \ueta p -\beta -\beta a \ueta q + {\bar w} \ueta(p- q)  \right ) \\
  && \hspace{30mm} + (\beta-\alpha) (a \ueta q + 1) + {\bar w} \ueta q  \Bigg )
\end{eqnarray*}}

\newpage
\twocolumn
